# Supplementary material for: Improving Hospital Mortality Prediction with Medical Named Entities and Multimodal Learning
Source: arXiv:1811.12276 source file (2018-12-04)
Supplement: Supplementary file 1 [file appendix_1.tex]

\begin{table}[htbp]
  \caption{Non-discharge Notes Statistics}
  \label{tab:notes}
  \centering 
  \begin{tabular}{lll}
  \toprule
    Category          &  \# of Notes in first 2 days & \# of Notes without timestamp in first 2 days \\ 
    \midrule
    Case Management   &  265    &  0  \\
    Consult           &  44     &  0  \\  
    ECG               &  34,021 &  34,021\\
    Echo              &  12,846 &  12,846 \\
    General           &  2,530  &  0 \\
    Nursing           &  56,250 &  0 \\ 
    Nursing/other     &  121,682&  0 \\
    Nutrition         &  1,482  &  0 \\
    Pharmacy          &  11     &  0 \\
    Physician         &  36,590 &  0 \\
    Radiology         &  127,916&  0 \\
    Rehab Services    &  496    &  0 \\
    Respiratory       &  5,121  &  0 \\ 
    Social Work       &  650    &  0 \\
    \midrule
    Total             &  399,904&  46,867  \\
  \bottomrule
  \end{tabular}
\end{table}
